# Supplementary material for: Affordance detection with Dynamic-Tree Capsule Networks
Source: arXiv:2211.05200 source file (2022-11-09)
Supplement: Supplementary file 1 [file appendix.tex]

\appendix
